# Supplementary material for: Weak ferromagnetism and short range polar order in NaMnF$_3$ thin films
Source: arXiv:1611.00845 source file (2017-02-06)
Supplement: Supplementary file 1 [file NMF_supplementary_5.pdf]

# Weak ferromagnetism and short range polar order in $NaMnF_3$ thin films

Supplementary Information


Amit KC,[1, 2] Pavel Borisov,[1] David Lederman,[1, 2] and Vladimir V. Shvartsman[3]

1) Department of Physics, West Virginia University, Morgantown, WV 26506, USA

2) Department of Physics, University of California, Santa Cruz, CA 95064, USA

3) Institute for Materials Science, University Duisburg-Essen, Universitatsstraβe 15, 45141 Essen, Germany


Here we present additional information regarding the growth and structure of the $NaMnF_3$ (NMF) samples. As mentioned in the manuscript, NMF thin films were grown on $SrTiO_3$ (001) single crystals and on $SrRuO_3$ films, 30 nm thick, also grown on STO (001). The x-ray diffraction reciprocal space maps (XRD RSMs) were obtained using a Rigaku SmartLab system mounted with a Ge (220) two-bounce monochromator incident optics. Because of the limitation of the SmartLab diffractometer, not all in-plane reflections obtained by rotating anode x-ray diffractometer were accessible for reciprocal space mapping.

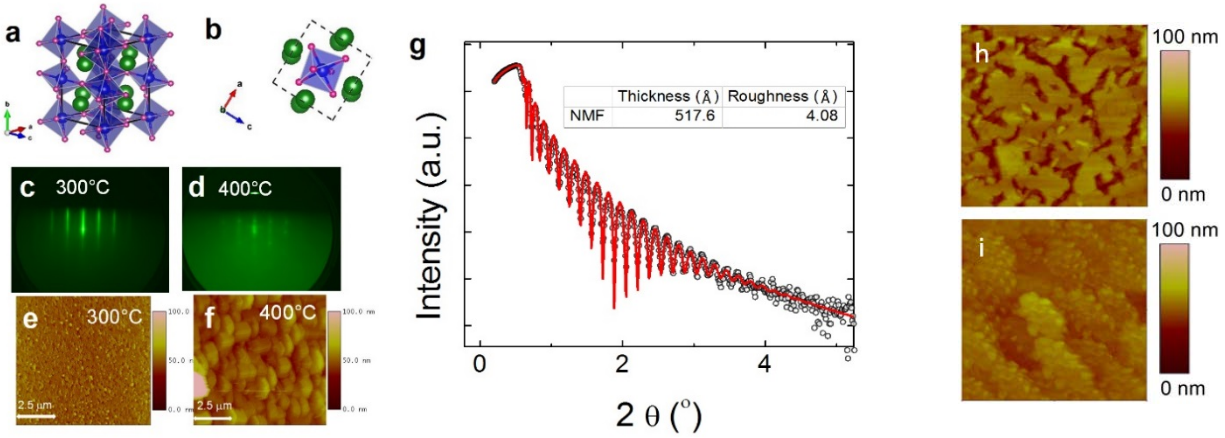


**Fig. S1** (a) Crystalline structure of $NaMnF_3$. (b) View of structure along the b-axis. (c-d) RHEED patterns for samples grown at 300 $^oC$ and 400 $^oC$ on STO. (e-f) AFM image of samples grown at 300 $^oC$ and 400 $^oC$ on STO. The sample becomes rougher with increasing growth temperature (g) X-ray reflectivity scan of 50 nm (nominal thickness) sample grown on STO (open circles) and the fit to the data using GenX software. The thickness and roughness parameters obtained from the fit are indicated in the figure. (h) & (i) AFM images, 2$\mu$m × 2 $\mu$m, of the NMF/STO and NMF/SRO samples surface respectively. The rms roughnesses of the images were 7.7 and 4.0 nm respectively.

The NMF thin films were grown via co-deposition of NaF (99.99%) and MnF 2 (99.99%) using commercial Knudsen cells. The fluxes of NaF (≈ 0.027 Å/s) and MnF 2 (≈ 0.043 Å/s) were measured using a quartz crystal monitor placed at the sample growth position. The growth was performed at substrate temperatures $T_s$ ranging from 200 °C to 450 °C in 50 °C steps, while the quality of the substrate and film

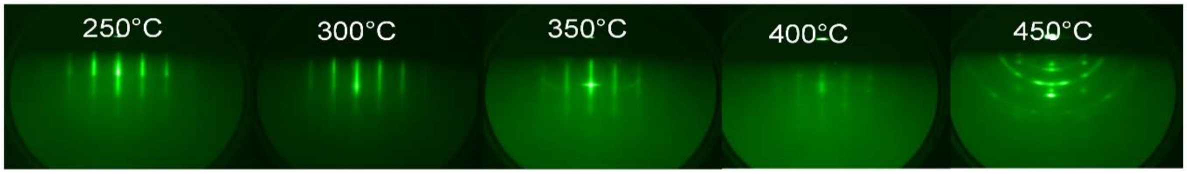


**Fig. S2** RHEED patterns obtained for the NMF sample grown at various substrate temperatures. Above 300 °C, the patterns become spottier and eventually circles appear at 450 °C. This indicates that the samples become rougher with increasing growth temperature, and eventually they become polycrystalline.

surfaces was monitored in-situ using reflection high energy electron diffraction (RHEED). Figure S1 shows RHEED and AFM data for NMF/STO samples grown at 300 °C and 400 °C, indicating the increasing roughness with growth temperature. The x-ray reflectivity of the sample grown at 300 °C indicates that the thickness was 51.8 nm and the roughness was 0.41 nm. The AFM image indicates that the surface was smooth over length scales of approximately 250 nm (Fig. S1h), but in the entire 2 μm × 2 μm image, the roughness is 7.7 nm because of the island structure of the topography.

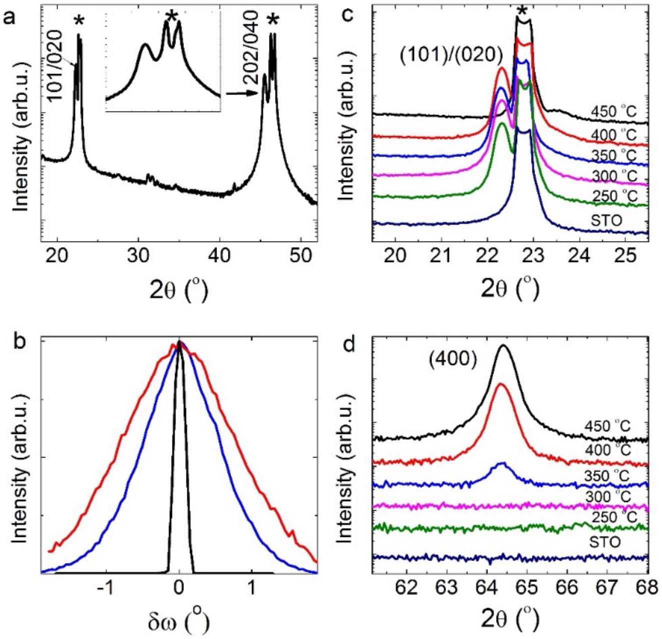


**Fig. S3** (a) XRD θ–2θ scan of the NMF/STO sample grown at 300 °C. The peaks marked with an asterisk belong to the (001), (002), and (003) STO substrate. The y-axis is logarithmic intensity. (b) Rocking curve of the STO around (100) peak (black), and of NMF/STO (blue) and NMF/SRO (red) around (101)/(020) peak. (c) Zoom of the NMF (202)/(040) peak grown

The RHEED patterns obtained after growth also indicate that the film surface and crystallinity degraded when the growth temperature was increased beyond 350 °C, as shown in Fig. S2. The x-ray

scans performed on samples grown at different temperatures, shown in Fig. S3, indicate that the crystalline degradation includes a re-orientation of the film along the [001] direction. Figure S3b shows the rocking curve of the NMF/STO and NMF/SRO grown at 300 $^{o}$C along with STO with a full width at half maximum (FWHM) of 1.32$^{o}$, 2.23$^{o}$ and 0.15$^{o}$, respectively. The relatively large rocking curve FWHM for the substrate is due to the instrument resolution.

As discussed in the text, only reflections from the orthorhombic phase of the film could be observed, indicating the absence of a $a = c$ distortion in the film. In addition, there were two NMF domains in the same film, one with $b_o$ in-plane and the other with $b_o$ out-of-plane which are referred as NMF(101) and NMF(010) domains respectively in the manuscript and supplementary information. Note that for the same plane, the angle $\chi$ (tilt angle with respect to surface normal) is different for NMF(010) and NMF(101) domains. This implies probing same plane of different NMF domains requires different tilts of sample stage before $\phi$, in-plane $\theta$–$2\theta$ and RSM scans. Figure S4a & b show the reciprocal space maps (RSMs) of the different domains. Figure S4a shows the reflection around the $(323)_o$ plane for $b_o$ in-plane i.e. NMF(101) domain, along with the (103) reflection from the substrate. Similarly, Fig. S4b shows the reflection around $(262)_o$ plane for $b$ out-of-plane i.e. NMF(010) domain, along with (203) reflection from the substrate. Furthermore, the presence of $(260)_o$ and $(062)_o$ reflections, as seen in Fig. S4c, and $(240)_o$ peak at 56.04 ± 0.05$^{o}$ and $(042)_o$ peak at 56.74 ± 0.05$^{o}$ (Fig. S5d) for NMF(010) domain show a difference in $a_o$ and $c_o$ lattice parameters confirming the orthorhombic nature of NMF(010) domain. The $(240)_o$ and $(042)_o$ peaks at 55.66 ± 0.02$^{o}$ and 56.95 ± 0.01$^{o}$ respectively (Fig. S5b) also confirm the absence of $a_o = c_o$ distortion for the NMF(010) domain. Figure S4d shows the out-of-plane RSM near the STO (002) reflection. Lattice parameters for each domains were obtained from the out-of-plane $\theta$–$2\theta$ scan of the $(040)_o/(202)_o$ reflection (Fig. 1a) and in-plane $\theta$–$2\theta$ scans of $(042)_o$ and $(222)_o$ reflections for corresponding domains in Fig. S5. Please refer to Table S1 for computed lattice parameters. For NMF(101) domains, the lattice parameters $a_o$ and $c_o$ had the same ≈2% strain but with opposite sign; that is, $a_o$ had a tensile strain

whereas $c_o$ had a compressive strain, while $b_o$ remained relaxed. It should be noted that the measured unit cell volume of 257 ± 2 Å$^3$ agrees with that of the bulk material (255.65 Å$^3$). For NMF(010) domains, all

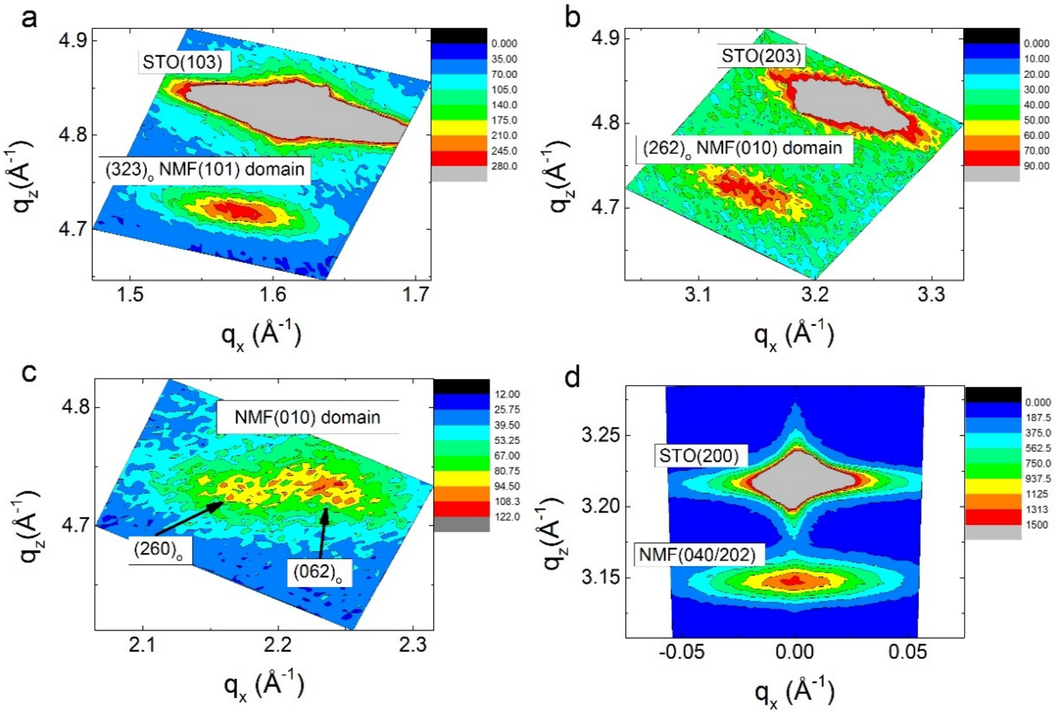


**Fig. S4 (**a) Reciprocal space map (RSM) around $(323)_o$ plane of NMF with (101) out-of-plane orientation, i.e. NMF(101) domain. (b) RSM around $(262)_o$ plane of NMF with (010) out-of-plane orientation i.e. NMF(101) domain. (c) RSM around $(260)_o$ and $(062)_o$ reflections of NMF(010) domain. (d) RSM around $(040)/(202)_o$ plane of NMF i.e. along the $q_z$ (out-of-plane orientation).

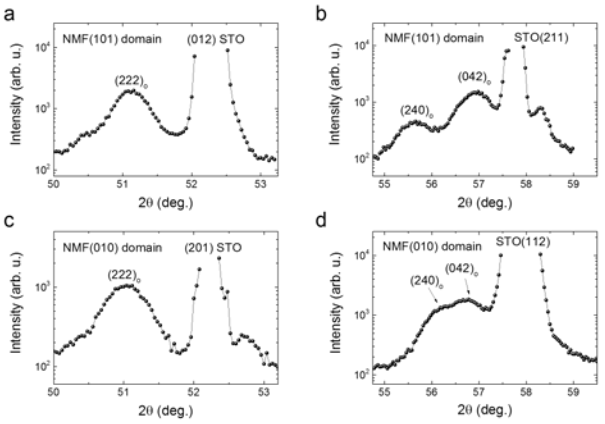


**Fig. S5 (**a) $\theta$–$2\theta$ scan around $(222)_o$ peak of NMF(101) domain with $\chi$ = 63.50˚. (b) $\theta$–$2\theta$ scan around $(042)_o$ peak of NMF(101) domain with $\chi$ = 65.09˚. (c) $\theta$–$2\theta$ scan around $(222)_o$ peak of NMF(010) domain with $\chi$ = 26.50˚. (d) $\theta$–$2\theta$ scan around $(042)_o$ peak of NMF(010) domain with $\chi$ = 35.82˚.

Table S1: Lattice parameters obtained from Fig. 1(a) and Fig. S5.

| | NMF(101) domain (Å) | NMF(010) domain (Å) | Bulk (Å) |
|---|---|---|---|
| a | 5.86±0.02 | 5.76±0.05 | 5.757 |
| b | 8.04±0.01 | 7.980±0.001 | 8.008 |
| c | 5.45±0.01 | 5.57±0.04 | 5.548 |

the lattice parameters were relaxed with a unit cell volume of 255± 2 Å$^3$. In Table S1 we also compare results from $b_o$ in-plane and the bulk lattice parameters from the literature (Ref. 14 of the manuscript). It appears that the $b_o$ in-plane domains are even more orthorhombic than the out-of-plane domains.

Since the magnetic signal from the film is small compared to that of the sample, a very careful analysis is needed. The temperature dependent magnetization measurements on NMF/STO were carried out by subtracting the magnetic background from the STO substrate under the same measurement conditions as described in the text. Figure S6a shows typical ZFC-FC and TRM (inset) curves obtained for precut 10×5×1 mm$^3$ STO(001) single crystal substrate after surface preparation process. The ZFC and FC curves (measured with $H$ = 1kOe applied in-plane along [001] same as sample) track each other without any significant splitting in the temperature range measured. The upturn at low temperatures (< 20 K) is most likely due to presence impurities in the substrate. The diamagnetic background slightly differed from one substrate to another, but the qualitative nature of ZFC, FC, and TRM curves remained the same. The

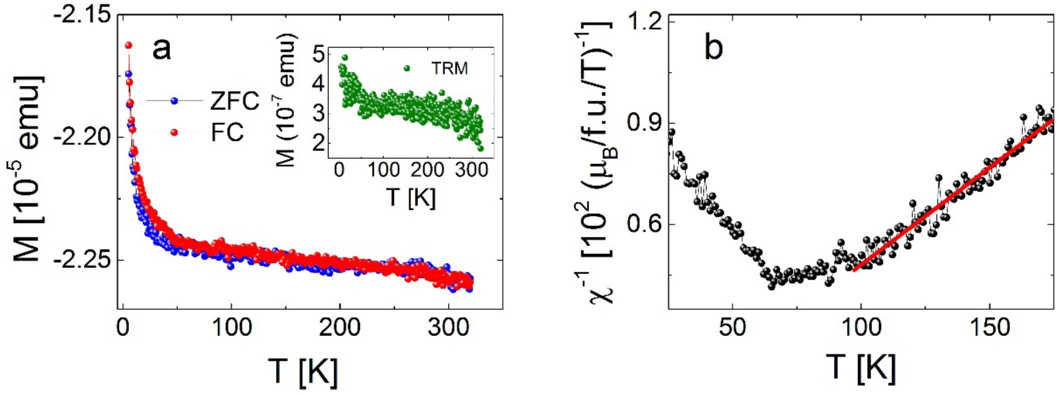


**Fig. S6** (a) Magnetic behavior of a precut 10×5×1 mm$^3$ STO(001) single crystal substrate after surface preparation process. (b) Inverse Magnetization M$^{-1}$ vs. T of NMF/STO sample. The straight red line is the Curie-Weiss fit for the ZFC data above the Neel temperature of the sample.

upturn in the ZFC and FC curves (Fig. 2a in the manuscript) at low temperatures (< 20 K) is mostly likely due to the impurities in the substrate and an imperfect background subtraction because of the reasons mentioned above.

The inverse magnetization vs. *T* for ZFC data is plotted on Fig. S6b. The diamagnetic background from the substrate was subtracted and a small offset of $4x10^{-7}$ emu was added to *m* in order to make data positive before taking inverse *m*. The straight red line is the best fit obtained using Curie-Weiss law [$\chi = C/(T - \theta)$] above $T_N$ which yielded Curie constant *C* and $\theta$ to be 1.63 $[\mu_B/(f.u.\cdot T\cdot K)]^{-1}$ and 18 ± 3 [K] respectively with coefficients of determination, $R^2 = 0.95$. This result is thus indicative of Curie-Wiess behavior of NMF film above the Neel temperature.
